# Supplementary material for: Towards More Economical Context-Augmented LLM Generation by Reusing Stored KV Cache
Source: arXiv:2503.14647 source file (2025-03-18)
Supplement: Supplementary file 1 [file 9-appendix_0525.tex]

\onecolumn % to fit tabularx 

\section*{Appendix.A Applications}
\label{sec:appendix}

\newcolumntype{L}{>{\small\arraybackslash}l}
\newcolumntype{C}{>{\small\arraybackslash}c}
\setlength\tabcolsep{1.5pt}
\begin{tabularx}{\linewidth}{|L|C|C|L|}
\caption{The statistics of 77 applications in empirical study. \footnotesize{(Multi-Choice-* refer to Multi-Choice (*-Order).)}} \label{tab:stats}\\ 
\hline
\multicolumn{1}{|C|}{\begin{tabular}[c]{@{}c@{}}\textbf{Application name}\\{(Link to Github repo)}\end{tabular}} & \multicolumn{1}{C|}{\begin{tabular}[c]{@{}c@{}}\textbf{Decision Type}\\{(Matching Order)}\end{tabular}} & \begin{tabular}[C|]{@{}c@{}}\textbf{\# of Target Classes} \\ (\# of labels per class)\end{tabular} & \multicolumn{1}{C|}{\begin{tabular}[c]{@{}c@{}}\textbf{Branch Conditions}\\(Class lists or value ranges are separated by semicolons.)\end{tabular}}\\ \hline 
\endfirsthead
\caption{The statistics of 77 applications in empirical study (Continued).}\\
\hline 
\multicolumn{1}{|C|}{\textbf{Application}} & \multicolumn{1}{C|}{\begin{tabular}[c]{@{}c@{}}\textbf{Decision Type}\\{(Matching Order)}\end{tabular}} & \begin{tabular}[C|]{@{}c@{}}\textbf{\# of Target Classes} \\ (\# of labels per class)\end{tabular} & \multicolumn{1}{C|}{\begin{tabular}[c]{@{}c@{}}\textbf{Branch Conditions}\\(Class lists or value ranges are separated by semicolons.)\end{tabular}}\\ \hline 
\endhead
\hline
\multicolumn{4}{r}{\footnotesize( To be continued )}
\endfoot
\hline
\endlastfoot

\multicolumn{4}{|C|}{Image Multi-Label Classification (Google \code{label\_detection}, AWS \code{detect\_labels})} \\ \hline
\href{https://github.com/spaceqorgi/2019-iot-ai-workshop}{2019-iot-ai-workshop}                    &   Multi-Choice-App                        & \textbf{2} (7, 2)                & [Capuchin monkey, ...]; [Wildlife biologist, ...]                                                          \\
\href{https://github.com/Grusinator/Aander-ETL}{Aander-ETL}                               &   Multi-Choice-App                        & \textbf{3} (9, 6, 5)             & [Landmark, Sculpture, ...]; [Building, Estate, ...]; [Human, ...]                                      \\
\href{https://github.com/SmartAppUnipi/ArtGuide}{ArtGuide}                                 &   Multi-Choice-API                            & \textbf{2} (6, 3)                & [Painting, Picture frame, ...]; [Building, Architecture, ...]                                              \\
\href{https://github.com/ShruthiAthikam/AWS_CloudComputing}{AWS\_CloudComputing}                      &  Multi-Select                           & \textbf{2} (1, 1)                & [Hot dog]; [Food]                                                                                          \\
\href{https://github.com/amruthasingh/DoorWatch}{AWS\_Rekognition}                   & True-False                               & \textbf{1} (6)                   & [Clothing, Person, Human, Furniture, Child, Man]                                                               \\
\href{https://github.com/Vickyilango/AWSRekognition}{AWSRekognition}                           &  Multi-Select                           & \textbf{2} (3, 3)                & [Person, People, Human]; [Art, Drawing, Sketch]                                                            \\
\href{https://github.com/hsunchi/GraduateProject}{GraduateProject}                             & True-False                               & \textbf{1} (5)                   & [Orator, Professor, Projection Screen, ...]                                                          \\
\href{https://github.com/Sarveshtg/-Voice-Assistant-for-Visually-Impaired}{Voice-Assistant}                       &  Multi-Select                           & \textbf{3} (5, 3, 1)          & [Highway, Lane, ...]; [Car, ...]; [Classroom]                                 \\
\href{https://github.com/julian-gamboa-ensino/callforcode}{callforcode}                              & True-False                               & \textbf{1} (5)                   & [Water, Waste, Bottle, Plastic, Pollution]                                                                     \\
\href{https://github.com/J-eld/AWS-Rekognition-Car-Image-search}{Car-Image-search}                        & True-False                               & \textbf{1} (6)                   & [Sedan, Mini SUV, Coupe utility, Truck, Van, Convertible]                                                      \\
\href{https://github.com/sanjay417/cloudComputing_project2}{cloudComputing\_project2}                          &   Multi-Choice-API                            & \textbf{3} (1, 3, 1)             & [Person]; [Dog, Cat, Mammal]; [Flower]                                                                 \\
\href{https://github.com/bhavani-goruganthu/CSC847_GAE_Proj2_VisionAPI}{CSC847\_GAE\_Proj2}                             &   Multi-Choice-API                            & \textbf{3} (2, 2, 1)             & [Mammal, Livestock]; [Human, People]; [Flower]                                                         \\
\href{https://github.com/cmonyeba/cutiehack}{cutiehack}                                &  Multi-Select                           & \textbf{2} (1, 3)                & [Banana]; [Lemon, Citrus fruit, Apple]                                                                     \\
\href{https://github.com/cloudwaysX/CycleGAN-tensorflow_pixie}{CycleGAN-tensorflow\_pixie}                          &   Multi-Choice-API                            & \textbf{3} (1, 6, 4)             & [Food]; [Girl, Boy, Man, ...]; [Room, Living room, House, ...]                                         \\
\href{https://github.com/CalvinKrist/DisasterRelief}{DisasterRelief}                           & True-False                               & \textbf{1} (8)                   & [Hurricane, Flood, Tornado, Landslide, Earthquake, Volcano, ...]                                               \\
\href{https://github.com/sun624/Dogecoin_musk}{Dogecoin\_musk}                           & True-False                               & \textbf{1} (4)                   & [Dog, Mammal, Carnivore, Wolf]                                                                                 \\
\href{https://github.com/desendoo/flaskAPI}{flaskAPI}                                & True-False                               & \textbf{1} (3)                   & [Food, Recipe, Ingredient]                                                                                     \\
\href{https://github.com/lyl0602/Cloud-based-automatic-food-assessment-system}{food-assessment-system}                  &  Multi-Choice-API                           & \textbf{5} (35, 22, 54, 4, 6)    & [Dessert, ...]; [Grilling, ...]; [Strawberries, ...]; [Cigarette, ...]; ...        \\
\href{https://github.com/pruthu-vi/CV-Project2/}{Foodier}                                  &  Multi-Select                           & \textbf{2} (13, 1)               & [Building, Logo, Menu, Person, Vehicle, People, ...]; [Food]                                               \\
\href{https://github.com/neeltron/Hack-At-Home-II}{Hack-At-Home-II}                          &   Multi-Choice-API                            & \textbf{2} (3, 3)                & [Food, Junk food, Plastic]; [Drinkware, Wood, Metal]                                                       \\
\href{https://github.com/matthew-chu/heapsortcypher}{HeapSortCypher}                           &   Multi-Choice-API                            & \textbf{3} (8, 5, 11)            & [Food, Food grain, ...]; [Clothing, Shirt, ...]; [Paper bag, ...]                                      \\
\href{https://github.com/laksh22/IngredientPrediction}{IngredientPrediction}                                &  Multi-Select                        & \textbf{3} (1, 1, 1)             & [Spaghetti]; [Bean]; [Naan]                                                                        \\
\href{https://github.com/mattheweis/FESMKMITL}{FESMKMITL}                                & True-False                               & \textbf{1} (1)                   & [Face]                                                         \\
\href{https://github.com/dafna1228/milab}{milab}                                  &   Multi-Choice-App                        & \textbf{3} (1, 1, 1)             & [Sign]; [Nature]; [Car]                                                                                \\
\href{https://github.com/gdsc-ssu/bird-sweeper}{BirdSwe}                         &   Multi-Choice-API                            & \textbf{1} (5)                & [Smoke, Bird, ...]                                                       \\
\href{https://github.com/BONITA-KWKim/ai-server-proto}{ai-server-proto}                      &   Multi-Choice-API                            & \textbf{3} (3, 14)                   & [Eye, Eyeball, Eyes]; [Landmark, Sculpture, Monument, ...]                                                                                                \\
\href{https://github.com/Flowmot1on/Phoenix}{Pheonix}                                  & True-False                               & \textbf{1} (1)                   & [Fire]                                                                                                         \\
\href{https://github.com/nina-mir/photo_book_google_app_engine}{photo\_book}                              &   Multi-Choice-API                            & \textbf{3} (10, 10, 2)           & [Mammal, Bird, Insect, ...]; [Skin, Lip, ...]; [Flower, Plant]                                         \\
\href{https://github.com/siwasu17/plant-watcher/}{Plant-Watcher}                            & True-False                               & \textbf{1} (5)                   & [Plant, Flowerpot, Houseplant, Bonsai, Wood]                                                                   \\
\href{https://github.com/hamzaish/RecycleBot}{RecBot}                               &   Multi-Choice-App                        & \textbf{2} (11, 8)               & [Tin, Paper, Magazine, Carton, ...]; [Food, Bread, Pizza, ...]                                             \\
\href{https://github.com/adrian-willi/roblab-hslu}{roblab-hslu}                              & True-False                               & \textbf{1} (7)                   & [Raincoat, Coat, Jacket, T-shirt, Trousers, Jeans, Shorts]                                                     \\
\href{https://github.com/kyu929/senior-project/}{senior-project}                           &   Multi-Choice-API                            & \textbf{3} (2, 3, 1)             & [Landscape, Landmark]; [Self-portrait, Portrait, ...]; [Flower]                                        \\
\href{https://github.com/ertheosiswadi/smart_can}{smart-can}                                & True-False                               & \textbf{1} (9)                   & [Paper, Bottle, Plastic, Container, Tin can, Glass, ...]                                                       \\
\href{https://github.com/cod-r/smart-trash-bin}{smart-trash-bin}                        &   Multi-Choice-API                            & \textbf{2} (14, 5)               & [Aviator sunglass, Beer glass, ...]; [Plastic arts, ...]                                                   \\
\href{https://github.com/yuvsc/smartHamper}{smartHamper}                              &   Multi-Choice-API                            & \textbf{3} (7, 4, 3)             & [Shirt, T-shirt, ...]; [Trousers, Denim, ...]; [Brand, Text, ...]                                      \\
\href{https://github.com/cmfabregas/StudySpaceAvailability}{StudySpaceAvailability}                   & True-False                               & \textbf{1} (4)                   & [Hardware, Power Drill, Drill, Electronics]                                                                    \\
\href{https://github.com/The-Coding-Kid/888hacks-flask}{The-Coding-Kid}                           &  Multi-Select                           & \textbf{6} (9, 6, 9, 3, 6, 3)    & [Noodle, ...]; [Meat, ...]; [Produce, ...]; [Fruit, ...]; [Milk, ...]; ... \\
\href{https://github.com/pankeshpatel/tinyml-computer-vision}{Tinyml}                  &  Multi-Select                           & \textbf{3} (4, 6, 5)             & [Car, Truck, ...]; [Gun, Weapon Violence, ...]; [Cat, Dog, ...]                                        \\
\href{https://github.com/yifei-tang/UofTHacksBackend}{UofTHacksBackend}                         &   Multi-Choice-API                            & \textbf{4} (3, 3, 7, 4)          & [T-shirt, ...]; [Outerwear, ...]; [Pants, ...]; [Footwear, ...]                                    \\
\href{https://github.com/gnawcire/garbage-sort}{garbage-sort}                          &   Multi-Choice-API                           & \textbf{2} (1, 20)    & [Food];[Metal, ...];          \\
\hline \hline
\multicolumn{4}{|C|}{Image Object Detection (Google \code{object\_localization})}\\\hline
\href{https://github.com/tjestes/equipment-detection-poc}{equipment-detection-poc}                  &  Multi-Select                          & \textbf{1} (1)                   & [Shoe]                                                                                                         \\
\href{https://github.com/nlonberg/flood-depths/}{flood\_depths}                            &  Multi-Select                           & \textbf{1} (5)                   & [Car, Van, Truck, Boat, Toy vehicle]                                                                           \\
\href{https://github.com/qwerty10w/SBHacks2021/}{SBHacks2021}                              &  Multi-Select                          & \textbf{1} (1)                   & [Person]                                                                                                       \\
\href{https://github.com/arosloff/SeeFarBeyond}{SeeFarBeyond}                             &  Multi-Select  & \textbf{1} (2)  & [Spoon, Coin]                                                                                                  \\
\href{https://github.com/thy0602/shecodes-hack}{shecodes-hack}                            &  Multi-Select                           & \textbf{1} (2)                   & [Dress, Top]                                                                                                   \\
\href{https://github.com/renilJoseph/SunHacks2019/}{SunHacks2019}                             &  Multi-Select                          & \textbf{1} (3)                   & [Person, Chair, Table]                                                                                         \\
\href{https://github.com/rlathgml/thgml/}{thgml}                                    &  Multi-Select                          & \textbf{1} (7)                   & [Pizza, Food, Sushi, Baked goods, Snack, Cake, Dessert]                                                        \\
\href{https://github.com/sarvesh-tech/Verlan/}{Verlan}                                   &  Multi-Select                        & \textbf{1} (2)                   & [Dog, Animal]                                                                                                  \\
\hline \hline
\multicolumn{4}{|C|}{Text Sentiment Classification (Google \code{sentiment\_detection})}\\\hline 
\href{https://github.com/OkapalDominic/animal_analysis}{animal-analysis}                          &   Multi-Choice-API                            & \textbf{4} (1, 1, 1, 1)          & [0.5, 1]; [0, 0.5]; [-0.5, 0]; [-1, -0.5]                                                          \\
\href{https://github.com/kmzjy110/calhacksv2}{calhacksv2}                               &   Multi-Choice-API                            & \textbf{6} (1, 1, 1, 1, 1, 1)    & [0.5, 1]; [0.5, 1]; [0.1, 0.5]; [-0.1, 0.1]; [-0.5, -0.1]; [-1, -0.5]                      \\
\href{https://github.com/steventhan/carbon-hack-sentiment}{carbon\_hack\_sentiment}                  &   Multi-Choice-API                            & \textbf{3} (1, 1, 1)             & [0.3333, 1]; [-0.3333, 0.3333]; [-1, -0.3333]                                                          \\
\href{https://github.com/Martincu-Petru/Cloud-Computing}{FoodDelivery}                         &   Multi-Choice-API                            & \textbf{3} (1, 1, 1)             & [0.6, 1]; [0.3, 0.6]; [-1, 0.3]                                                                        \\
\href{https://github.com/ryanphennessy/devfest}{devfest}                                   &   Multi-Choice-API                            & \textbf{4} (1, 1, 1, 1)          & [0.6, 1]; [0.4, 0.6]; [0.2, 0.4]; [-1, 0.2]                                                        \\
\href{https://github.com/ChainZeeLi/EC601_twitter_keyword}{EC601\_twitter\_keyword}                  &   Multi-Choice-API                            & \textbf{3} (1, 1, 1)             & [0.25, 1]; [-0.25, 0.25]; [0.25, 1]                                                                    \\
\href{https://github.com/Dacs95/ElectionSentimentAnalysis}{ElectionSentimentAnalysis}                 &   Multi-Choice-API                            & \textbf{3} (1, 1, 1)             & [0.05, 1]; [0, 0.05]; [-1, 0]                                                                          \\
\href{https://github.com/jtkrumlauf/Hapi}{Hapi}                                        &   Multi-Choice-API                            & \textbf{2} (1, 1)                & [-1, 0]; [0, 1]                                                                                            \\
\href{https://github.com/beekarthik/JournalBot}{JournalBot}                               &   Multi-Choice-API                            & \textbf{3} (1, 1, 1)             & [0.5, 1]; [0, 0.5]; [-1, 0]                                                                            \\
\href{https://github.com/whtai/Mind-Reading-Journal/}{Mind\_Reading\_Journal}                   &   Multi-Choice-API                            & \textbf{4} (1, 1, 1, 1)          & [0.15, 1]; [0.1, 0.15]; [-0.15, 0.1]; [-1, -0.15]                                                  \\
\href{https://github.com/Mrkr1sher/Sarcatchtic-MakeSPP19}{Sarcatchtic-MakeSPP19}                  &   Multi-Choice-API                            & \textbf{2} (1, 1)                & [-0.5, 1]; [-1, -0.5]                                                                                      \\
\href{https://github.com/nicholasadamou/stockmine}{stockmine}                                &   Multi-Choice-API                            & \textbf{2} (1, 1)                & [-1, 0]; [0, 1]                                                                                            \\
\href{https://github.com/KijanaG/Tone}{Tone}                                     &   Multi-Choice-API                            & \textbf{3} (1, 1, 1)             & [-1, -0.5]; [-0.5, 0.5]; [0.5, 1]                                                                      \\
\href{https://github.com/nixin72/UOttaHack-2019}{UOttaHack\_2019}                          &   Multi-Choice-API                            & \textbf{3} (1, 1, 1)             & [0.25, 1]; [-0.25, 0.25]; [-1, -0.25]                                                                  \\
\hline \hline
\multicolumn{4}{|C|}{Text Entity Detection (Google \code{entity\_detection})}\\\hline
\href{https://github.com/Jhuynh760/GeoScholar}{GeoScholar}                               & True-False                               & \textbf{1} (1)                & [LOC]                                                                                   \\
\href{https://github.com/mihirKachroo/HackThe6ix}{HackThe6ix}                               &   Multi-Choice-API                            & \textbf{7} (1, 1, 1, 1, 1, 1, 1) & [PERSON]; [LOC]; [ADD]; [NUM]; [DATE]; [PRICE]; [ORG]             \\
\href{https://github.com/dev5151/Klassroom}{Klassroom}                                &   Multi-Choice-API                            & \textbf{2} (2, 2)                & [PERSON, PROPER]; [LOC, ORG]                                                                 \\
\href{https://github.com/da1234/newsChronicle/}{newsChronicle}                            & True-False                               & \textbf{1} (1)                   & [OTHER]                                                                                                        \\
\href{https://github.com/larry852/ocr-contratos/}{ocr-contratos}                           & True-False                               & \textbf{1} (1)                   & [NUM]                                                                                                          \\
\href{https://github.com/AllegraChen/uofthacks6}{uofthacks6}                               & True-False                               & \textbf{1} (1)                   & [OTHER]                                                                                                        \\
\hline \hline
\multicolumn{4}{|C|}{Text Topic Classification (Google \code{text\_classify})} \\ \hline
\href{https://github.com/Shrinjay/DMnMD}{DMnMD}                                    & True-False                               & \textbf{1} (1)                   & [Health]                                                                                                       \\
\href{https://github.com/saheedandrew/HLPFL}{HLPFL}                                    & True-False                               & \textbf{1} (8)                   & [Public Safety, Law \& Government, Emergency Services, News, ...]                                              \\
\href{https://github.com/SaiManukonda/MirrorDashboard}{MirrorDashboard}                          & True-False                               & \textbf{1} (7)                   & [Jobs \& Education, Law \& Government, News, ...]                                                              \\
\href{https://github.com/GalenWong/noteScript}{noteScript}                               & True-False                               & \textbf{1} (1)                   & [Food]                                                                                                         \\
\href{https://github.com/dwang/pennapps-2019f}{pennapps\_2019f}                          & True-False                               & \textbf{1} (2)                   & [News/Politics, Investing]                                                                                     \\
\href{https://github.com/jcavejr/soap}{soap}                                     &   Multi-Choice-API                            & \textbf{2} (2, 2)                & [Sensitive Subjects, ...]; [Discrimination \& Identity Relations, ...]                                     \\
\href{https://github.com/Samvit123/SocialEyes-MakeSPP2018}{SocialEyes}                               &   Multi-Choice-API                            & \textbf{2} (2, 1)                & [people \& society, sensitive subjects]; [adult]                                                           \\
\href{https://github.com/gpesma/Twitter-Mining-GAE}{Twitter\_Mining\_GAE}                     & True-False                               & \textbf{1} (1)                   & [Sentitive]                                                                                                    \\
\href{https://github.com/JoosepAlviste/vfriendo}{vfriendo}                                 & True-False                               & \textbf{1} (1)                   & [Restaurants]                                                                             
\end{tabularx}

\twocolumn % to fit tabularx 

\section*{Appendix.B Loss function for other \summaries}
\label{sec:loss_appendix}

 \mypara{\term{True-False}}

\begin{align}
     L(y) &= \overbrace{ \textrm{Sigmoid}(\max_{\LabelId \in \TargetSet_{\hat{\ClassId}}}(\y) - \theta)
}^{\substack{\text{\sf \footnotesize {Penalize {\bf Type-1} Critical Errors}} 
}} \nonumber \\&+
\overbrace{ \textrm{Sigmoid}(\theta-\max_{\LabelId \in \TargetSet_{\ClassId}}(\y))
}^{\substack{\text{\sf \footnotesize {Penalize {\bf Type-1} Critical Errors}} 
}} 
\end{align}

\mypara{\term{Multi-Select}}
\begin{equation}
\begin{aligned}
     L(y) &= \overbrace{ \sum_{\ClassId \in \hat{T}}\textrm{Sigmoid}(\theta - \max_{\LabelId \in \TargetSet{\ClassId}} \y[\LabelId] )
}^{\substack{\text{\sf \footnotesize {Penalize {\bf Type-1} Critical Errors}} 
}} \\
&+\overbrace{ \sum_{\ClassId \in \cup_{\ClassId} \TargetSet_{\ClassId} \setminus \hat{T}}\textrm{Sigmoid}(\max_{\LabelId \in \TargetSet{\ClassId}} \y[\LabelId] - \theta)
}^{\substack{\text{\sf \footnotesize {Penalize {\bf Type-3} Critical Errors}} 
}} 
\end{aligned}
\end{equation}

\mypara{\term{Multi-Choice API-order}}
Here we explain why this loss function captures the critical errors:
\begin{packeditemize}
    \item A Type-1 error occurs, if (1) the correct \target is matched, thus at least one of its labels has a score above the confidence threshold ($\max_{\LabelId \in \TargetSet_{\hat{\ClassId}}} \y[\LabelId] \geq \theta$), and (2) it is matched after the EOD because all of the labels belonging to the correct \target have scores below the maximum score of labels in the incorrect \targets. 
    \item A Type-2 error occurs if the maximum score for labels in a correct \target falls below threshold $\theta$, thus it is never matched (before or after EOD).
    \item A Type-3 error occurs if any labels belonging ($\max_{\LabelId \notin \TargetSet_{\hat{\ClassId}}} \y[\LabelId]$) to  incorrect \targets appears before labels in the correct \target. 
    
\end{packeditemize}

\cc{The equation contains two ``type-2''}
\begin{equation}
\begin{aligned}
     L(\y) &=   
  \overbrace{ \textrm{Sigmoid}\left(\max_{\LabelId \in \cup_{\ClassId \neq \hat{\ClassId} }\TargetSet_{\ClassId}}\y[\LabelId] - \max_{\LabelId \in \TargetSet_{\hat{\ClassId}}} \y[\LabelId]\right) }^{\substack{\text{\sf \footnotesize {{\bf Type-1} Critical Errors}} }} \\
  &+
  \overbrace{ \textrm{Sigmoid}\left(\max_{\LabelId \in \cup_{\ClassId \neq \hat{\ClassId} }\TargetSet_{\ClassId}}\y[\LabelId] - \theta\right)}^{\substack{\text{\sf \footnotesize {{\bf Type-2} Critical Errors}} }}\\
  &+
  \overbrace{ \sum_{\ClassId \neq \hat{\ClassId}}\textrm{Sigmoid}\left( \max_{\LabelId \in \TargetSet_{\ClassId}}\y[\LabelId] 
- \max_{\LabelId \in \TargetSet_{\hat{\ClassId}}}\y[\LabelId] \right)}^{\substack{\text{\sf \footnotesize {{\bf Type-3} Critical Errors}} }}
  \label{eq:loss_app2}
\end{aligned}
\end{equation}

\mypara{\term{Value ranges}} As for APIs that output a score $\y$ to describe the input, applications typically define several value ranges as target classes to make decisions, where the lower bound of the $\ClassId^{th}$ \target is denoted as $l_\ClassId$ and the upper bound of the $\ClassId^{th}$ \target is denoted as $u_\ClassId$. 

\begin{equation}
\begin{aligned}
L(y_i) &= 
\overbrace{ \textrm{Sigmoid}\left(\y - u_{\hat\ClassId} \right) +
\textrm{Sigmoid}\left(l_{\hat\ClassId}- \y \right)  }^{\substack{\text{\sf \footnotesize {{\bf Type-1} Critical Errors}} }} \\&+
\overbrace{ \sum_{\ClassId \neq \hat{\ClassId}} \textrm{Sigmoid}(u_{\ClassId} - \y) + \textrm{Sigmoid}(\y - l_{\ClassId} ) }^{\substack{\text{\sf \footnotesize {{\bf Type-3} Critical Errors}} }} 
 \label{eq:value}
\end{aligned}
\end{equation}
where $\hat{\ClassId}$ is the index of the correct \target. 
A Type-1 error occurs (\ie a correct \target is matched after EOD) when the output score $\y$ exceeds the upper bound of the ground-truth value range ($u_{\ClassId}$), or falls below the lower bound of the ground-truth value range ($l_{\ClassId}$).
A Type-3 error occurs when the upper bound of an incorrect value range exceeds $\y$ \emph{and} its lower bound falls below $\y$, leading it to be selected. 
Type-2 errors are absent in this application because all the \targets span the whole output range, thus a \target must be matched.

% Similar to the idea of the loss function we construct for classification tasks, compared to the Mean Squared Error loss which penalizes the score $y_i$ if it is not equal to the ground truth,  \tool's proposed loss function only penalizes the score if it falls out of the range that ground truth lies in. 
% % MSE loss, borrow the idea 
 
% \yh{1. correct w/ low scores before break, 2. correct w/ low score after break but higher than theta 3. incorrect with high score before break}

% \mypara{\term{Multi-Select}}As for \term{Multi-Select} decision, multiple selections are allowed about which target class(es) the ML API output matches with. In this case, the decision process will not break until encountering a \target whose \score is lower than $\theta$. An incorrect decision may be made when the target classes selected by ground-truth decision are ranked after the break at $\theta$, or when target classes not selected by ground-truth decision are ranked before the break at $\theta$. Thus, we penalize the type-2 critical errors and type-3 critical errors by assigning $\theta$ as the values for $\F(y)$ and $\Q(y)$. 
