# Supplementary material for: Towards More Economical Context-Augmented LLM Generation by Reusing Stored KV Cache
Source: arXiv:2503.14647 source file (2025-03-18)
Supplement: Supplementary file 2 [file revision-appendix.tex]

\onecolumn % to fit tabularx 

\section*{Appendix. }
\label{sec:revision}

\section*{Labels included in each subcategory} 

\subsection{}
